# Supplementary material for: Improved Gradient based Adversarial Attacks for Quantized Networks
Source: arXiv:2003.13511 source file (2021-12-29)
Supplement: Supplementary file 1 [file advtrain_supp++.tex]

% \begin{table*}[!h]
% \centering
% % \vspace{0mm}
% % \begin{center}
% \scriptsize
% \begin{tabular}{l|ccc}
% \toprule
%  \multirow{2}{*}{Methods} & \multirow{2}{*}{\acrshort{FGSM}} & \multicolumn{2}{c}{ \acrshort{FGSM++}} \\
%  & & \acrshort{HNS} & \acrshort{IGNS} \\
 
% % \multirow{2}{*}{Methods} & \multicolumn{3}{c}{\acrshort{FGSM}} \\ 
% %  & \acrshort{ORIG.} & \acrshort{HNS} & \acrshort{JSVS-GT} \\
% \midrule

% \acrshort{REF} & 62.38 & \textbf{61.40} & 61.42 \\
% \acrshort{BC} \cite{courbariaux2015binaryconnect} & 53.91 & 52.27 & \textbf{52.19} \\
% \acrshort{GD}-$\tanh$ \cite{ajanthan2019mirror} & 56.13 & \textbf{54.81} & 54.84 \\
% \acrshort{MD}-$\tanh$-\acrshort{S} \cite{ajanthan2019mirror} & 55.10 & \textbf{53.82} & 53.84 \\
% % \acrshort{BNN-WAQ} \cite{hubara2016binarized} &  &  &    \\
% \bottomrule
% \end{tabular}
% \caption{\em Adversarial accuracy on the test set for adversarially trained floating and binary neural networks using different methods for quantization using Original $L_\infty$ bounded \acrshort{FGSM} attack and \acrshort{FGSM++} attack with \acrshort{HNS} and \acrshort{IGNS}.}
% \label{table:advtrain_supp++}
% \end{table*}

\begin{table*}[!h]
\centering
% \vspace{0mm}
% \begin{center}
\scriptsize
\begin{minipage}[c]{0.37\linewidth}    
\begin{tabular}{l|ccc}
\toprule
 \multirow{2}{*}{Methods} & \multirow{2}{*}{\acrshort{FGSM}} & \multicolumn{2}{c}{ \acrshort{FGSM++}} \\
 & & \acrshort{HNS} & \acrshort{IGNS} \\
 
% \multirow{2}{*}{Methods} & \multicolumn{3}{c}{\acrshort{FGSM}} \\ 
%  & \acrshort{ORIG.} & \acrshort{HNS} & \acrshort{JSVS-GT} \\
\midrule

\acrshort{REF} & 62.38 & \textbf{61.40} & 61.42 \\
\acrshort{BC} \cite{courbariaux2015binaryconnect} & 53.91 & 52.27 & \textbf{52.19} \\
\acrshort{GD}-$\tanh$ \cite{ajanthan2019mirror} & 56.13 & \textbf{54.81} & 54.84 \\
\acrshort{MD}-$\tanh$-\acrshort{S} \cite{ajanthan2019mirror} & 55.10 & \textbf{53.82} & 53.84 \\
% \acrshort{BNN-WAQ} \cite{hubara2016binarized} &  &  &    \\
\bottomrule
\end{tabular}
\end{minipage}\hfill
\begin{minipage}[c]{0.62\linewidth}
\caption{\em Adversarial accuracy on the test set for adversarially trained floating and binary neural networks using different methods for quantization using Original $L_\infty$ bounded \acrshort{FGSM} attack and \acrshort{FGSM++} attack with \acrshort{HNS} and \acrshort{IGNS}.}
\label{table:advtrain_supp++}
\end{minipage}
\end{table*}

    % \begin{tabular}{ll|cc}
    %     \toprule
    %     &Algorithm & \cifar{-10} & \cifar{-100}\\
    %     \midrule
    %     &\acrshort{REF} (float) & $93.67$ & $73.97$ \\ 
    %     &\acrshort{BC} & $86.84$ & $65.04$ \\
    %     \midrule
    %     \parbox[t]{2mm}{\multirow{2}{*}{\rotatebox[origin=c]{90}{Ours}}}
    %     &\acrshort{MD}-$\softmax$-\acrshort{S} & $89.71$ & $66.40$ \\ 
    %     &\acrshort{MD}-$\tanh$-\acrshort{S} & $\textbf{89.99}$ & $\textbf{66.63}$ \\
    %     \bottomrule
    % \end{tabular}
    % \end{minipage}\hfill
    % \vspace{-2ex}
    % \caption{\em Classification accuracies on the test for \smobilenet{V2} where all the learnable parameters are binarized.
    % Our stable \acrshort{MD} variants significantly outperformed \acrshort{BC} while \acrshort{MD}-$\tanh$-\acrshort{S} is slightly better than \acrshort{MD}-$\softmax$-\acrshort{S} in these cases.
    % }
    % \label{tab:res_mobilenet_bracewell}
